# Supplementary material for: New physics footprints in the angular distribution of $B_s\to D_s^*(\to D_s\gamma,\,D_s\pi)\, \tau\, \nu$ decays
Source: arXiv:2110.05526 source file (2021-10-11)

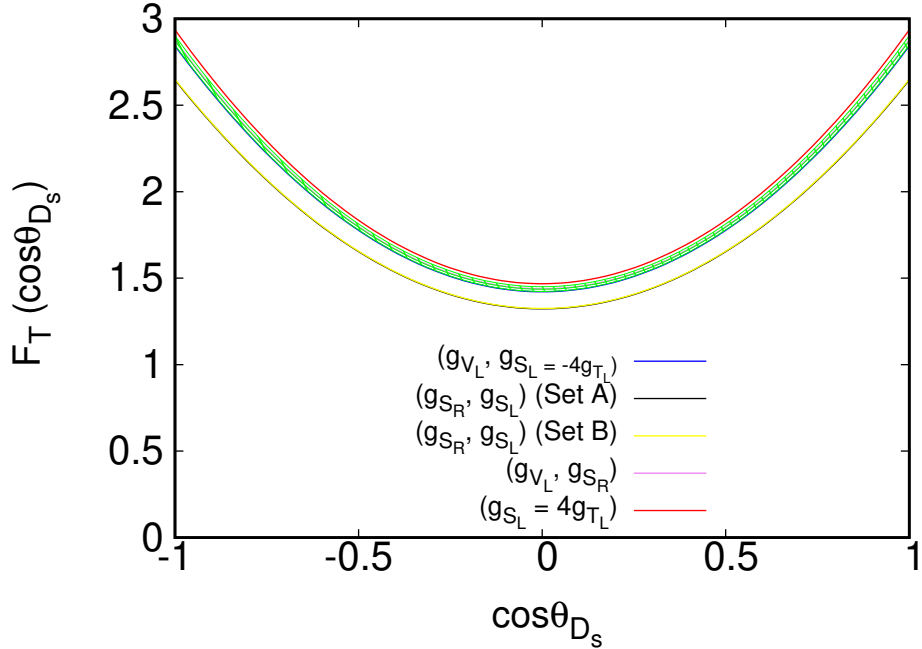

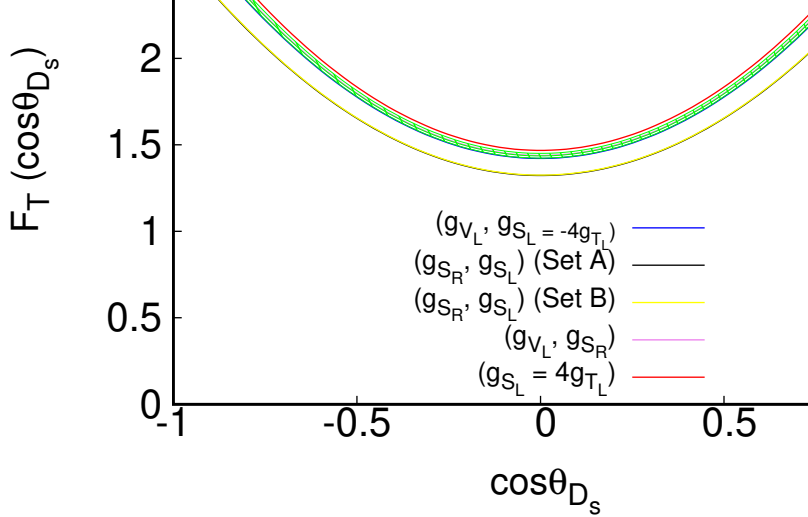

Supplement: Supplementary file 66 [file q2_dsg_zft_c0v_sm_Sc2-eps-converted-to.pdf]
